# Supplementary material for: Logarithmic Upturn in Low-Temperature Electronic Transport as a Signature of d-Wave Order in Cuprate Superconductors
Source: arXiv:1811.12348 ancillary file (2018-11-29)
Supplement: Supplementary file 1 [file ZhouSIOpt.pdf]

# Logarithmic Upturn in Low-Temperature Electronic Transport as a Signature of d-Wave Order in Cuprate Superconductors Supplementary Material

Xiaoqing Zhou,[1,2] D. C. Peets,[3,4] Benjamin Morgan,[5] W. A. Huttema,[1] N. C. Murphy,[1] E. Thewalt,[1] C. J. S. Truncik,[1] P. J. Turner,[1] A. J. Koenig,[1] J. R. Waldram,[5] A. Hosseini,[3] Ruixing Liang,[3,6] D. A. Bonn,[3,6] W. N. Hardy,[3,6] and D. M. Broun[1,6]

[1]*Department of Physics, Simon Fraser University, Burnaby, BC, V5A 1S6, Canada*
[2]*Department of Physics, University of Colorado, Boulder 80309-0390, USA*
[3]*Department of Physics and Astronomy, University of British Columbia, Vancouver, BC, V6T 1Z1, Canada*
[4]*State Key Laboratory of Surface Physics, Department of Physics, and Advanced Materials Laboratory, Fudan University, Shanghai 200433, People's Republic of China*
[5]*Cavendish Laboratory, Madingley Road, Cambridge, CB3 0HE, United Kingdom*
[6]*Canadian Institute for Advanced Research, Toronto, Ontario, MG5 1Z8, Canada*

## S1. EXPERIMENTAL METHODS

### A. Cavity perturbation measurements

Microwave surface impedance was measured using cavity perturbation [1, 2] of high quality factor $TiO_2$ (rutile) dielectric resonators [3, 4]. The use of normal-metal (copper) enclosures allowed the dielectric resonators to be operated in strong static magnetic fields up to 8 T, while the high dielectric constant and low loss tangent of rutile give quality factors of $10^6$ to $10^7$ for the empty resonator. Multiple configurations of the resonator were used, with the majority of the data measured with cavities excited in the $TE_{011}$ mode at frequencies ranging from 2.5 to 5.5 GHz. In addition, three higher order modes of one of the resonators were used to study the frequency dependence of the vortex dynamics, up to 14 GHz. Single crystal samples were mounted on sapphire or silicon "hot fingers" [5] with a small quantity of vacuum grease and were introduced into the dielectric resonators through holes bored along the cylinder axes of the resonators. A microwave magnetic field $H_{\rm rf}$, regulated to have fixed field strength in order to avoid nonlinear effects, was applied perpendicular to the $CuO_2$ planes, to induce in-plane screening currents of constant magnitude. The presence of the small sample perturbatively reduced the resonator volume and shifted the resonant frequency $f_0$. In addition, the sample dissipation reduced the resonator quality factor and increased the resonant bandwidth $f_{\rm B}$. On the basis of these effects, the surface impedance $Z_{\rm s} = E_{||}/H_{||} = R_{\rm s} + {\rm i}X_{\rm s}$, was obtained using the cavity perturbation formula [1, 3, 6]

$$R_{\rm s}(B,T) + {\rm i}\Delta X_{\rm s}(B,T) = \Gamma\left(\frac{\Delta f_{\rm B}(B,T)}{2} - {\rm i}\Delta f_0(B,T)\right) . \quad \text{(S1)}$$

Here $R_{\rm s}(B,T)$ is the absolute surface resistance, at magnetic field $B$ and temperature $T$; $\Delta X_{\rm s}(B,T)$ is the change in surface reactance with respect to zero field and base temperature; $\Delta f_{\rm B}(B,T)$ is the change in resonator bandwidth on inserting the sample, relative to the empty resonator at zero field; $\Delta f_0(B,T)$ is the frequency shift with respect to zero field and base temperature; and $\Gamma$ is an empirically determined resonator constant. The absolute surface reactance was determined either using published penetration depth data [7] or, for the lower $T_{\rm c}$ samples, by imposing the Hagen–Rubens condition, $R_{\rm s} = X_{\rm s}$, in the normal state [1]. The absolute surface impedance is equivalent to the complex resistivity $\tilde\rho$ and conductivity $\sigma$ through

$$Z_{\rm s} = \sqrt{{\rm i}\mu_0\omega\tilde\rho} = \sqrt{{\rm i}\mu_0\omega/\sigma} \quad \text{(S2)}$$

in the local electrodynamic limit. In other words, we directly measure the effective complex resistivity

$$\tilde\rho = \frac{Z_s^2}{{\rm i}\mu_0\omega}. \quad \text{(S3)}$$

All measurements were carried out in the field-cooled state, except for field-swept data on $NbSe_2$, which were taken to reproduce conditions employed in corresponding DC experiments in the literature. Experiments were carried out in two different cryostats: a $^4$He cryostat [3], with a base temperature of 1.1 K; and a $^3$He–$^4$He dilution refrigerator [8], in which the sample could be cooled to 0.1 K. Measurements were carried out in the linear response regime, and self-heating effects were checked for and avoided. A worst-case estimate places an upper bound of 2 Å on the amplitude of the vortex motion, with typical displacements much less than 1 Å [4], much smaller than the inter-vortex spacing, of order 100 Å.

Examples of raw surface impedance data for optimally doped $YBa_2Cu_3O_{6.93}$ are presented in Fig. S1 for magnetic fields $B = 0$, 1, 2 and 4 T, at a measurement fre-

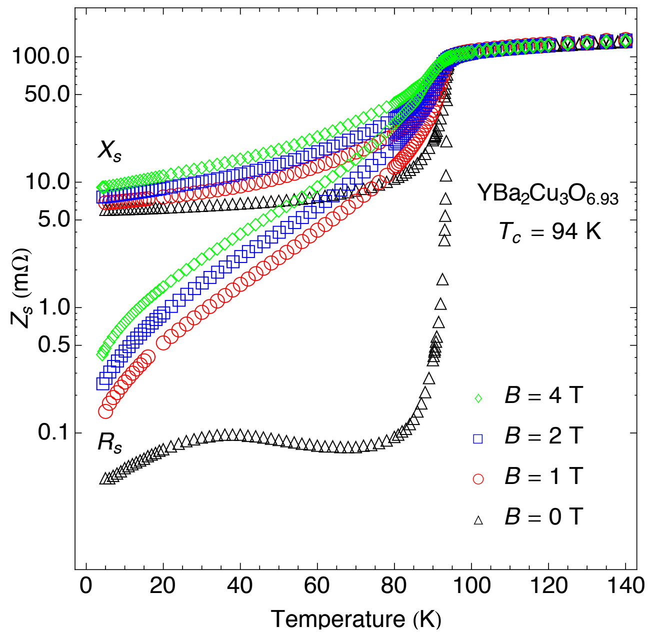


FIG. S1: Microwave surface impedance data for optimally doped $YBa_2Cu_3O_{6.93}$, measured at 5.49 GHz using cavity perturbation of a dielectric resonator. In zero field, $R_s(T)$ displays a characteristic low temperature peak, indicative of the very long quasiparticle lifetimes in this material [2, 9–11]. Surface resistance increases rapidly with the application of magnetic field, showing that vortex contributions to dissipation dominate over quasiparticle processes in the superconducting medium between the vortices. All measurements have been made in the field-cooled state, in order to nucleate a near-equilibrium vortex configuration.

quency $\omega/2\pi = 5.49$ GHz. Note that even in zero applied field (the Meissner state) the surface impedance of the superconductor is finite — the inertia of the superelectrons requires significant electric fields to drive the oscillating currents that screen the microwave fields from the interior of the sample. The surface impedance is predominantly reactive in this regime, with $X_s$ roughly two orders of magnitude larger than $R_s$ in zero field. The zero-field surface resistance of $YBa_2Cu_3O_{6.93}$ carries a characteristic signature of the quasiparticle physics — a low temperature peak in $R_s(T)$ due to a rapid increase in quasiparticle lifetime on cooling through $T_c$. Such peaks are wiped out by impurity scattering, and are therefore only observed in the highest quality samples [2, 9–11].

The application of a magnetic field fills the sample with vortices and establishes the flux-line lattice. Its impact can clearly be seen in the data on $YBa_2Cu_3O_{6.93}$ in Fig. S1. In particular, $R_s$ increases by one to two orders of magnitude when vortices are added to the superconductor, making the subtraction procedure (see below) used to isolate the vortex resistivity particularly robust.

### B. Extraction of vortex parameters

When a transport current density $J_0$ is driven through a type-II superconductor in the vortex state, the current exerts a Lorentz force $J_0\Phi_0$ per unit length on the flux lines, where $\Phi_0$ is the superconducting flux quantum. If the flux lines are free to move in response to the current, their motion will induce electric fields in the vicinity of the vortex cores, which couple to charge excitations in the superconductor — either bound states inside the cores or extended quasiparticle states outside the cores — and give rise to resistive dissipation. The flux-flow resistivity, $\rho_{\rm ff}$, is defined so that the power dissipation per unit volume is $P_v = \rho_{\rm ff} J_0^2$. Alternatively, the dissipation can be represented by a vortex viscosity $\eta$, defined so that the power dissipation per unit length of flux line is $P_\ell = \eta v^2$, where $v$ is the vortex velocity. These two representations can be related by considering force balance in the steady state. Equating the power dissipation per unit volume in the two cases then leads to the relation

$$\rho_{\rm ff} = B\Phi_0/\eta \, , \qquad \text{(S4)}$$

where $B$ is the magnetic induction.

In any real superconductor, local material inhomogeneities lead to pinning, preventing the free flow of flux lines. Since the displacement of the flux lines $x$ is very small relative to the inter-vortex spacing in our measurement, we can characterize the pinning effect as a linear restoring force $F = -\alpha x$ where $\alpha$ is the pinning constant. Pinning effects can be particularly strong in the cuprate superconductors, especially at low temperatures, making DC flux-flow resistivity difficult to measure. One approach is to use a DC current that exceeds the critical current to push the vortices into a state of free flux-flow. However, this is a nonlinear method and must be applied and interpreted carefully, and its use in cuprate superconductors is rare.

An alternative approach, which we employ, is to probe the *linear* response of the vortices to a high frequency driving current. This shakes the flux lines harmonically about their equilibrium positions, with a displacement that is small compared to the inter-vortex spacing. When carried out at frequencies in the GHz range, viscous and elastic forces become comparable in magnitude [12]. Since, as shown below, viscous and elastic forces occur 90° out of phase, this contactless, phase-sensitive technique allows the dissipative and pinning forces to be directly and separately resolved, without encountering the nonlinearities found in the DC technique.

When the Lorentz force is balanced by both viscous and elastic forces we obtain the following dynamical model [4, 12–14],

$$\eta v + \alpha x = \Phi_0 j(t) \, , \qquad \text{(S5)}$$

where $v = \dot{x}$. (As discussed in Refs. 15 and 4, it is not necessary to include a vortex Hall effect under conditions of constant driving current, which is the case appropriate to the microwave measurements.) For a time harmonic driving current, $j(t) = \mathrm{Re}\left\{J_{\mathrm{rf}}\mathrm{e}^{\mathrm{i}\omega t}\right\}$, the equation of motion can be recast in the frequency domain as

$$\left(\eta(\omega) + \frac{\alpha(\omega)}{\mathrm{i}\omega}\right)\tilde{v}\mathrm{e}^{\mathrm{i}\omega t} = \Phi_0 J_{\mathrm{rf}}\mathrm{e}^{\mathrm{i}\omega t}\;, \tag{S6}$$

which describes a massless, driven, damped harmonic oscillator. Together, $\eta$ and $\alpha$ determine the phasor vortex velocity,

$$\tilde{v} = \frac{\Phi_0 J_{\mathrm{rf}}}{\eta(\omega) + \alpha(\omega)/\mathrm{i}\omega}\;, \tag{S7}$$

which is the steady-state response to the driving current. This in turn governs the time rate of change of magnetic flux associated with vortex motion and, via the Josephson relation for moving vortices [16], the average electric field

$$\tilde{E} = B\tilde{v} = \frac{B\Phi_0}{\eta(\omega) + \alpha(\omega)/\mathrm{i}\omega}J_{\mathrm{rf}} \equiv \tilde{\rho}_v J_{\mathrm{rf}}. \tag{S8}$$

The coefficient relating electric field to applied current is the complex vortex resistivity, $\tilde{\rho}_v$, which represents the vortex contribution to resistivity. The flux-flow resistivity, $\rho_{\mathrm{ff}}$, is the zero-pinning limit of the vortex resistivity, $\rho_{\mathrm{ff}} = B\Phi_0/\eta$. In the presence of pinning it can be extracted using

$$\rho_{\mathrm{ff}}^{-1} = \mathrm{Re}\{\rho_v^{-1}\} = \frac{\mathrm{Re}\{\rho_v\}}{|\rho_v|^2}\;. \tag{S9}$$

Similarly, the pinning constant can be extracted using

$$\alpha = \omega B\Phi_0 \mathrm{Im}\{-\rho_v^{-1}\} = \omega B\Phi_0 \frac{\mathrm{Im}\{\rho_v\}}{|\rho_v|^2}\;. \tag{S10}$$

This is not the entire story, however, as we should also take into account the finite contribution of the superconducting background medium in which the vortices are embedded, even though it is usually not particularly prominent, as can be seen in Fig. S1. Coffey and Clem [17] and Brandt [18] have shown that the effect of inserting vortices into a pristine superconductor is to a good approximation additive in the effective resistivity

$$\tilde{\rho}_{\mathrm{eff}} \simeq \tilde{\rho}_{\mathrm{s}} + \tilde{\rho}_{\mathrm{v}} = \tilde{\rho}_{\mathrm{s}} + \frac{B\Phi_0}{\eta(\omega) + \alpha(\omega)/\mathrm{i}\omega}\;. \tag{S11}$$

Therefore, in this work $\tilde{\rho}_v$ was extracted from the difference between the in-field complex resistivity $\tilde{\rho}_{\mathrm{eff}}(B)$ and the zero-field complex resistivity $\tilde{\rho}_{\mathrm{s}}(0)$. This is expected to be a very good approximation in the limit $B \ll B_{c2}$.

### C. Samples

Microwave flux-flow impedance measurements were made on a series of high quality single crystals of $YBa_2Cu_3O_{6+y}$ and $Tl_2Ba_2CuO_{6+\delta}$ prepared at the University of British Columbia. The $YBa_2Cu_3O_{6+y}$ samples were grown by a self-flux method in nonreactive $BaZrO_3$ crucibles and have cation disorder at the $10^{-5}$ level [19]. Oxygen content was set by annealing in ultra-pure, ultra-dry flowing oxygen at temperatures between 350 °C (overdoped) and 914 °C (underdoped). For the most underdoped material ($y = 0.333$) the high temperature oxygen anneal was followed by a homogenization anneal at 570 °C in a sealed quartz ampoule [20]. This is the same sample as used in Refs. 21 and 22. As in that work, high pressure annealing (30 kbar) at room temperature was used to increase $T_{\mathrm{c}}$ from 3 K to 16 K. The $YBa_2Cu_3O_{6.52}$ sample, a small platelet single crystal, was mechanically detwinned and Ortho-II ordered, and is the same sample as used in Ref. 4. In order to confirm that sample morphology (surface roughness and demagnetizing factor) is not an important consideration in the microwave flux-flow experiments, for one of the dopings (optimal doping) results for two very different geometries were compared. The first optimally doped sample was cut from a thick, twinned $YBa_2Cu_3O_{6.93}$ single crystal and shaped into a plate 0.42 mm long in the $c$ direction and 0.93 mm × 0.080 mm in the $ab$ plane. This sample had a low demagnetizing factor in our experimental geometry. The second optimally doped sample was a naturally untwinned platelet measuring $a\times b\times c = 0.89\ \mathrm{mm}\times 0.72\ \mathrm{mm}\times 0.024\ \mathrm{mm}$, resulting in a large demagnetizing factor. The two samples gave very similar results, in particular displaying the same minimum in flux-flow resistivity at $T = 13$ K. However, data on the second sample were only taken down to $T = 5$ K and so are not reported here. The final $YBa_2Cu_3O_{6+y}$ sample was a mechanically detwinned, platelet crystal with $y = 0.993$, $T_{\mathrm{c}} = 89$ K, and Ortho-I oxygen ordering.

In order to carry out further measurements in the overdoped regime, samples of $Tl_2Ba_2CuO_{6+\delta}$ were used. These were grown by a copper-oxide-rich self-flux method in $Al_2O_3$ crucibles, using a time-varying encapsulation scheme [23]. The $T_{\mathrm{c}} = 45$ K crystal was annealed in a 1% $O_2$–$N_2$ gas flow at 480 °C for 16 days. The $T_{\mathrm{c}} = 25$ K crystal was annealed in pure flowing oxygen at 500 °C for 10 days. The samples were embedded in $Tl_2Ba_2CuO_{6+\delta}$ powder and placed in small quartz test-tubes during the anneals, which were quenched in an ice-water bath at the end of the runs to ensure good oxygen homogeneity. Both $Tl_2Ba_2CuO_{6+\delta}$ samples were small platelets, thin in the $c$ direction.

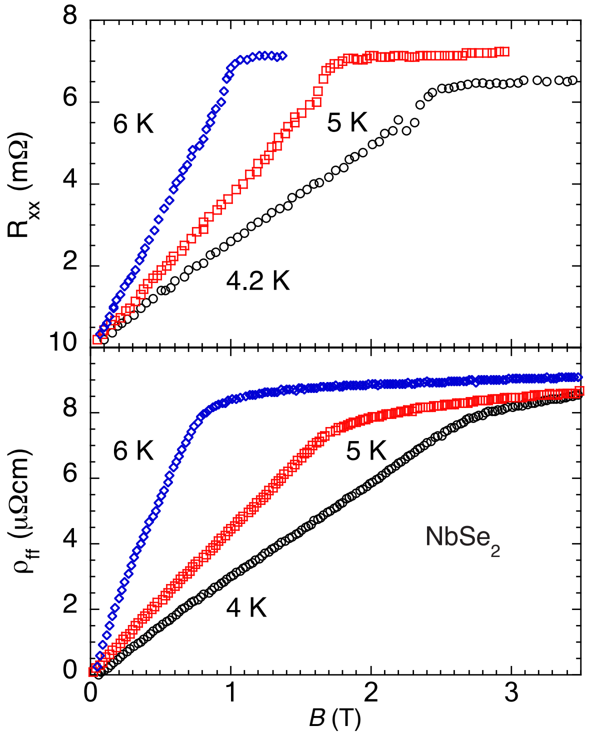


FIG. S2: Comparison of DC flux-flow resistance (upper panel, from Ref. 24) and our 2.79 GHz microwave flux-flow resistivity (lower panel) in $NbSe_2$ single crystals. In both cases the data were taken at constant temperature, in field-swept mode.

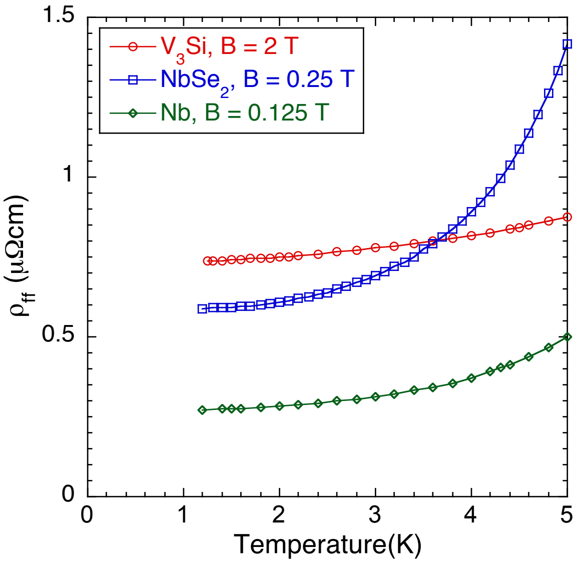


FIG. S3: Microwave flux-flow resistivity of Nb, $NbSe_2$ and $V_3Si$ measured at 2.79 GHz, showing monotonic temperature dependences, flattening out at low temperatures.

## S2. COMPATIBILITY WITH EXISTING KNOWLEDGE

### A. Case study: flux-flow resistivity in conventional superconductors

To the best of our knowledge, our work is the first to systematically study the complete vortex-dynamical response across the entire superconducting phase in the cuprate phase diagram, with a focus on the connection between flux-flow resistivity and normal state resistivity. That, and the difficulty to measure flux-flow resistivity directly in cuprates, means that the majority of our results have no suitable precedents to be directly compared with. On the other hand, flux-flow resistivity has been studied extensively in conventional superconductors, for which the Bardeen–Stephen relation is well established.

To demonstrate the reliability of microwave measurements of flux-flow resistivity, we have taken data on conventional superconductors for which DC measurements are available in the literature. In the first case, shown in Fig. S2, we compare the microwave flux-flow resistivity of a $NbSe_2$ single crystal with DC measurements by Bhattacharya *et al.* on the same material [24]. The microwave data were obtained under similar conditions to the DC experiments: at constant temperature, with varying magnetic field (field-swept mode). The Bhattacharya *et al.* data were published as raw resistances rather than as resistivities, so are subject to an unknown scaling factor. Modulo the uncertainty in scale, the two data sets can be overlaid and agree very well in field and temperature dependence.

In Fig. S3 we show the temperature dependence of flux-flow resistivity in three conventional superconductors: Nb, $NbSe_2$ and $V_3Si$. Note, in particular, the monotonic temperature dependence of $\rho_{ff}$, which flattens out at low temperatures as expected from Bardeen–Stephen theory, reflecting the weak temperature dependences of the normal-state resistivity and upper critical field in this temperature range.

Overall, we find our flux-flow resistivity measurements on conventional superconductors to be consistent with existing knowledge such as the Bardeen–Stephen law. However, this is in sharp contrast to our new findings on cuprate superconductors, implying that the vortex dynamics in cuprates are indeed very different.

### B. Case study: flux-flow resistivity and pinning on optimally doped $YBa_2Cu_3O_{6+x}$ extracted from DC measurements

As mentioned above, it is extremely challenging to extract and interpret DC flux-flow resistivity in cuprate superconductors. To the best of our knowledge, the only DC flux-flow resistivity measurements available are for

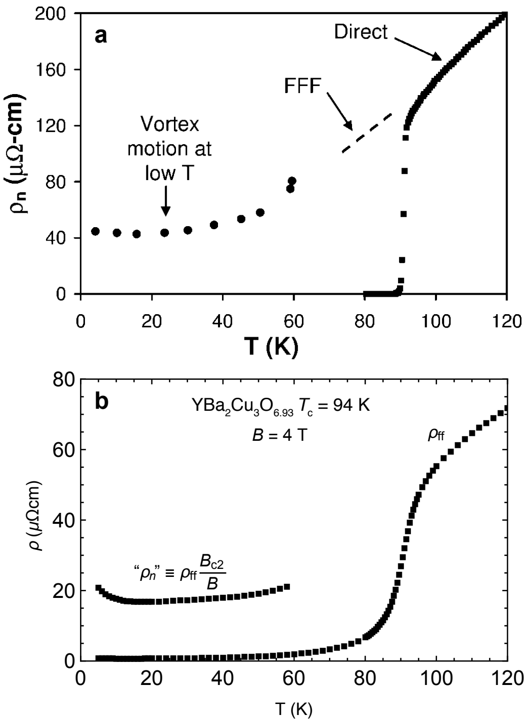


FIG. S4: a) "Normal state resistivity" obtained by scaling DC flux-flow measurements on optimally doped $YBa_2Cu_3O_{6+x}$ by an assumed vortex-core fraction, reprinted from reference [25]. Strong current pulses were used to overcome pinning and achieve flux flow. b) Microwave flux-flow resistivity measurements of optimally doped $YBa_2Cu_3O_{6.93}$, scaled in the same way as a), by a factor of $B_{c2}(T)/B$.

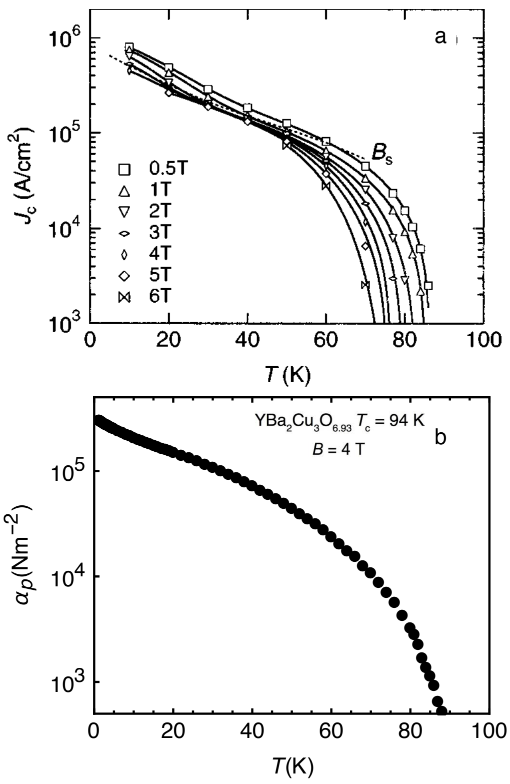


FIG. S5: a) Critical current density $J_c$ of an optimally doped $YBa_2Cu_3O_{6+x}$ sample, extracted from DC magnetization measurements, reprinted from reference [26]. b) Pinning constant $\alpha_p$ extracted from our microwave measurements on an optimally doped $YBa_2Cu_3O_{6.93}$ sample. The two quantities can be related through the force balance equation, in which the Lorentz force per unit length at critical current $J_c\Phi_0$ overcomes the pinning force $\alpha_p x$, where $\Phi_0$ is the flux quantum and $x$ is the maximum displacement of flux from its equilibrium position.

an $YBa_2Cu_3O_{6+x}$ film with $T_c = 91$ K [25], made using a very large current density in the MA/cm$^2$ range, in order to overcome pinning. Assuming that the Bardeen–Stephen law remains valid for cuprates, the authors scaled their flux-flow resistivity measurements by an assumed vortex-core fraction to obtain a "normal state resistivity" $\rho_n \equiv \rho_{ff} B_{c2}/B$, with their results reprinted in Fig. S4a. We stress that the results from our current work disagree with this conventional interpretation. Nevertheless, for the purposes of comparison, we have followed their procedure and performed a similar scaling of the microwave flux-flow resistivity of optimally doped $YBa_2Cu_3O_{6.93}$, with the results shown in Figure S4b. It can be seen that the two data sets are rather similar. Although the authors of the DC flux-flow study argued that their "normal state resistivity" was metallic (i.e., resistance decreasing with decreasing temperature) over a large portion of the temperature range, we note that on closer inspection of their data there appears to be a weak upturn at low temperature. While this upturn was previously overlooked, it coincides with our observations of weak flux-flow resistivity upturns in the optimally doped and overdoped samples.

Since flux-flow resistivity and pinning constant are two sides of the same coin in our measurement, we can also make qualitative comparisons between microwave pinning-constant measurements and the critical current density extracted from DC magnetization measurements on a $T_c = 91.6$ K sample [26], as shown in Figure S5. In spite of the difference in the techniques, the overall phenomenology is rather similar. This is expected, as the pinning constant should be roughly proportional to the critical current density in a DC measurement. In both cases, an exponential temperature dependence can be observed in the low temperature range, and at a melting temperature $T_m$ the pinning constant/critical current starts to drop quickly.

Overall, the strong resemblance between vortex parameters determined by DC and microwave techniques gives us a great deal of confidence in the validity of the microwave approach.

### C. Case study: previous high frequency measurements on cuprates

We also compare our results with previous high frequency determinations of vortex parameters in cuprates, made at microwave and terahertz frequencies. It is worth noting from the outset that both flux-flow resistivity and pinning constant are in general frequency-dependent response functions, as discussed in Ref. 4. This can be understood as analogous to the frequency-dependent Drude conductivity of a metal: microscopically, the conductivity and viscosity arise from the scattering of quasiparticles, the transport relaxation rate of which sets a natural frequency scale (or distribution of scales). Quasiparticle relaxation rates in clean cuprate samples are typically in the microwave range, meaning that we expect conductivities and viscosities measured at microwave frequencies to have similar magnitudes to DC values, but to generally be somewhat larger than in the THz range. This is borne out by the data.

For the Ortho-II $YBa_2Cu_3O_{6.52}$ sample we have probed vortex dynamics at 4 different microwave frequencies, allowing a stringent test of the vortex dynamics model against constraints imposed by causality. A detailed analysis and discussion has been presented in Ref. 4, which we summarize here:

1. The vortex viscosity $\eta(\omega)$ (dissipative response) of ultra-clean Ortho-II $YBa_2Cu_3O_{6.52}$ has strong frequency dependence in the microwave range. Via the associated Kramers–Kronig relation this implies a frequency dependence of the effective pinning constant $\alpha_{\rm eff}(\omega)$ (reactive response), which is indeed observed (see Fig. S6, reprinted from Ref. 4). This is a strong validation of the technique/analysis.
2. The vortex viscosity, plotted in Fig. S7a, has very similar frequency and temperature dependence to the zero-field quasiparticle conductivity, $\sigma_1(\omega, T)$, plotted in Fig. S7b. In particular, the narrow viscosity and conductivity spectra indicate relaxation rates in the low microwave range, with the characteristic temperature peaks a signature of the rapid collapse of inelastic scattering on cooling into the superconducting state. For the conductivity $\sigma_1(\omega, T)$ these effects are well understood in terms of long-lived nodal quasiparticles of the clean $d$-wave superconductor. Their appearance in $\eta(\omega, T)$ is then strong evidence that quasiparticle states *outside* the vortex cores provide the dominant damping mechanism for vortex motion, via their interaction with the electrical fields induced by the motion of the flux-line (illustrated in Fig. 1c).
3. By revealing the intrinsic, strong frequency dependence of $\eta(\omega)$ and $\alpha(\omega)$ in the microwave range, we are well placed to compare with other experiments, by extrapolation down to DC, and up into the THz range.

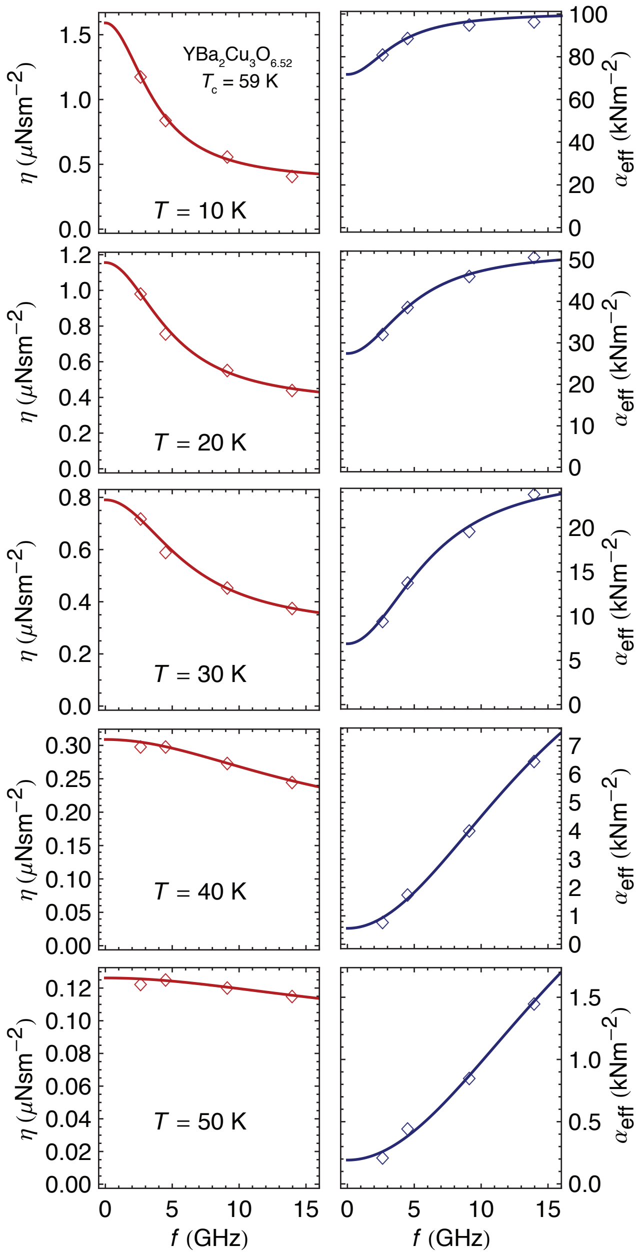


FIG. S6: Vortex viscosity $\eta(\omega)$ (left-hand column) and pinning constant $\alpha_{\rm eff}(\omega)$ (right-hand column) for Ortho-II $YBa_2Cu_3O_{6.52}$, reprinted from Ref. 4, for four microwave frequencies, at $B = 4$ T. Solid curves are simultaneous Kramers–Kronig fits to $\eta(\omega)$ and $\alpha_{\rm eff}(\omega)$, showing excellent consistency with constraints imposed by causality. The extracted vortex parameters can be extrapolated in this way to both DC and THz limits.

In general, $\eta(\omega)$ is a decreasing function of frequency, and we expect microwave measurements of viscosity to be similar to those in the DC limit, but to be substantially higher than the viscosity in the THz range, via the relaxation effects responsible for the frequency dependence.

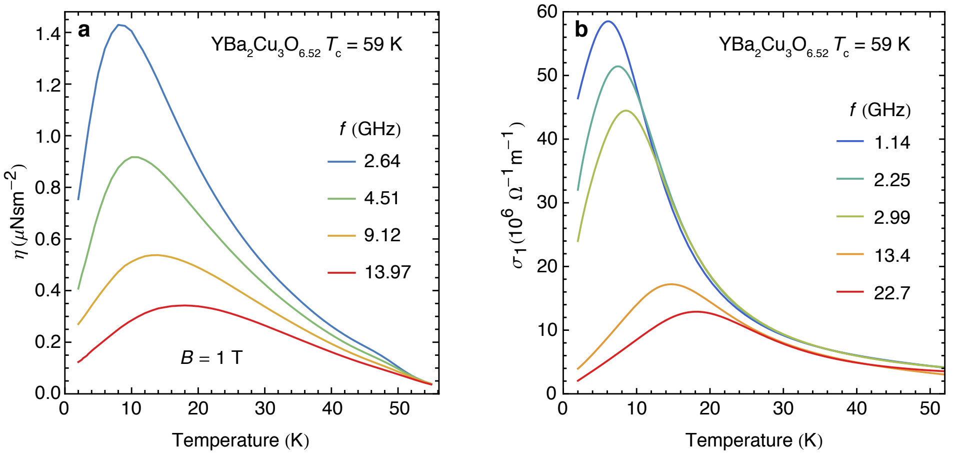


FIG. S7: Comparison of a) $B = 1$ T vortex viscosity of Ortho-II $YBa_2Cu_3O_{6.52}$ from Ref. 4 with b) zero-field quasiparticle conductivity for Ortho-II $YBa_2Cu_3O_{6.52}$ (geometric mean of $a$ and $b$-axis conductivity from Ref. 27).

Similar, $\alpha(\omega)$ is an increasing function of frequency, so measurements of pinning in the low microwave range will be comparable to but somewhat larger than DC values. Measurements of $\alpha$ in the high microwave range typically extrapolate well to THz values. This, again, is in broad agreement with experiment.

A figure from the microwave study by Tsuchiya *et al.* in Ref. 28, carried out on a $T_c = 91$ K $YBa_2Cu_3O_{6+x}$ sample, is reprinted in Figure S8a for comparison to our own results in Figure S8b. The overall trend is very similar in both cases, but with our experiment providing more closely spaced data points and higher resolution. Interestingly, the low temperature part of the Tsuchiya *et al.* viscosity data hints at a downturn in viscosity coefficient at low temperature, as revealed very clearly in our experiment. The magnitude of the viscosity coefficient in Ref. 28, measured in the high microwave range, is several times smaller than our data at 5.5 GHz. This is in line with the results from Ortho-II $YBa_2Cu_3O_{6.52}$ discussed previously, which showed that $\eta(\omega)$ is a decreasing function of frequency in the microwave range.

Terahertz data on vortex pinning constant, from Ref. 29, along with measurements of vortex viscosity, made on three $YBa_2Cu_3O_{6+x}$ films with $T_c$ between 85 and 88 K, are reprinted in Fig. S9a and S9b and compared with our microwave data on optimally doped $YBa_2Cu_3O_{6.93}$. Despite major differences in technique and frequency range, there is good qualitative agreement between the THz and microwave data. The magnitude and temperature dependence of the pinning constant is very similar and, within experimental uncertainty, the shape of $\eta(T)$ is consistent, with a suggestion of non-monotonic temperature dependence also appearing in the terahertz data. The difference in magnitude of vortex viscosity is again in line with the intrinsic frequency dependence of $\eta$ revealed in our earlier study on Ortho-II $YBa_2Cu_3O_{6.52}$ [4].

In conclusion, our extracted vortex data on optimally doped and overdoped $YBa_2Cu_3O_{6+x}$ samples are consistent with existing results in the literature, with new features revealed by the higher resolution. In the viscos-

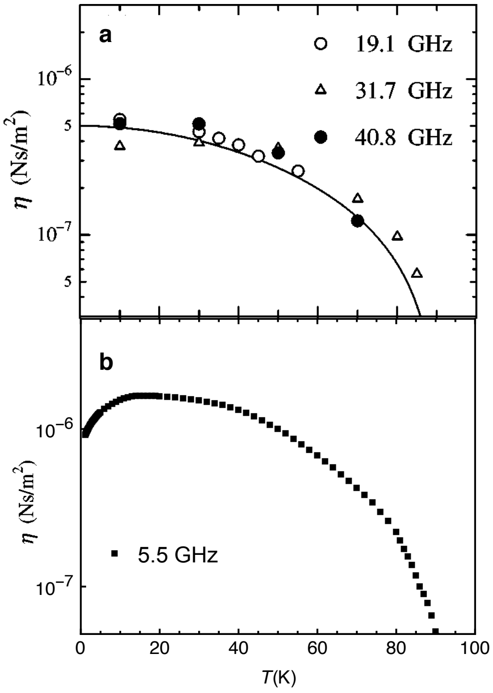


FIG. S8: a). Microwave measurements of vortex viscosity on a $T_c = 91$ K $YBa_2Cu_3O_{6+x}$ sample by Tsuchiya et al. [28], compared with b) our vortex viscosity measurements on a $YBa_2Cu_3O_{6+x}$ sample of similar doping made at a lower microwave frequency (5.5 GHz).

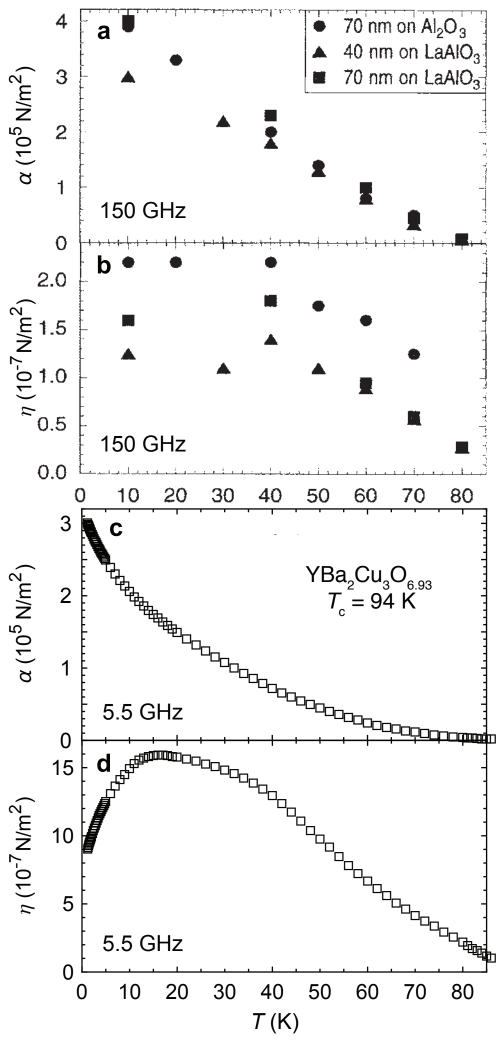


FIG. S9: a) Vortex pinning constant $\alpha$ and b) vortex viscosity $\eta$ extracted from terahertz measurements [29] of vortex response on three $YBa_2Cu_3O_{6+x}$ films, compared with our microwave measurements of c) vortex pinning constant and d) vortex viscosity on a single crystal of $YBa_2Cu_3O_{6+x}$ of similar doping.

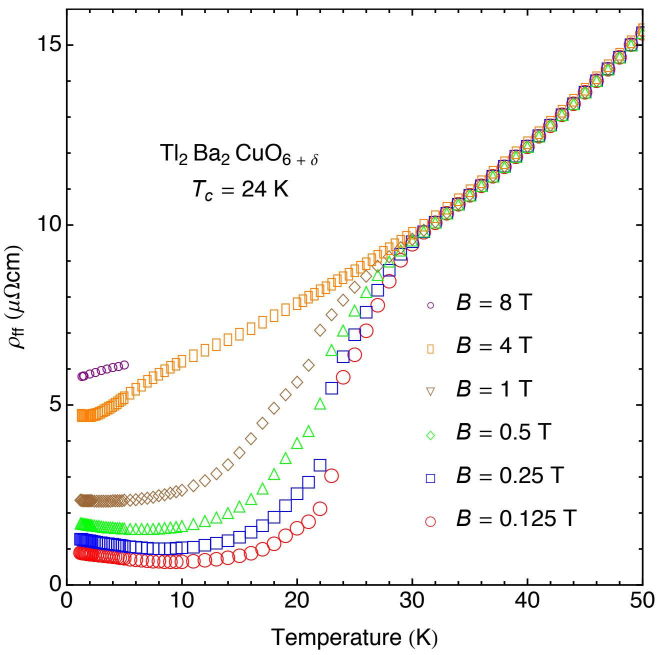


FIG. S10: Flux-flow resistivity of a highly overdoped sample of $Tl_2Ba_2CuO_{6+\delta}$ with $T_c = 24$ K. Low field data at $B = 0.125, 0.25$ and 0.5 T all show clear upturns below 10 K. This gradually transitions by $B = 8$ T to the monotonic temperature dependence of the normal state.

ity in particular, the older data appear to be on the verge of resolving the peak in $\eta(T)$ that is responsible for the main finding of the current work, the $\log(1/T)$ upturn in flux-flow resistivity.

### D. Case study: field-recovered normal state resistivity and flux-flow resistivity on strongly overdoped $T_c$ =24 K $Tl_2Ba_2CuO_{6+\delta}$

It is known that for highly overdoped cuprate samples, a Fermi-liquid-like $T^2$ temperature dependence of resistivity at low temperatures can be recovered using relatively low magnetic fields to destroy the superconducting order. It would then be expected for such a sample that the temperature dependence of flux-flow resistivity should gradually evolve from the $\log(1/T)$ form into the $T^2$ normal state resistivity with increasing field, since in the normal state $\rho_{\rm ff} \to |\rho_2^2 + \rho_1^2|/\rho_1 \approx \rho_1$. Since the evolution happens over a regime in which $B \ll B_{c2}$ no longer holds, we have to take into account the volume-exclusion effect of the vortex cores, by assuming that the superconducting background contribution to the effective complex resistivity scales as $\tilde{\rho}_s(B = 0) \times (1 - B/B_{c2}(T))$, where for concreteness $B_{c2}(T)$ follows a conventional BCS form.

Here we present the extracted flux-flow resistivity of our most overdoped sample, $T_c = 24$ K $Tl_2Ba_2CuO_{6+\delta}$, in magnetic fields up to 8 T. As shown in Fig. S10, the negative temperature slope at low temperatures gradually weakens as magnetic field increases, and a positive temperature dependence is recovered at low temperature at the highest field of 8 T. This apparent breakdown of the Bardeen–Stephen relation is consistent with our proposal that the $\log(1/T)$ form is directly related to the existence of vortices, which are absent in the field-recovered normal state on the overdoped side of the phase diagram.

**Acknowledgments**

The $V_3Si$ crystal used as a conventional-superconductor test sample was grown by Dr. Bernd Seeber at the Université de Genève [30] and cut and polished by Dr. Chris Bidinosti at the University of British Columbia. The $NbSe_2$ test sample was a crystal grown by Dr. Joseph Brill at the University of Kentucky and previously used in $\mu$SR measurements [31].

[1] O. Klein, S. Donovan, M. Dressel, and G. Gruner, Int. J. Inf. Milli. **14**, 2423 (1993).
[2] D. M. Broun, W. A. Huttema, P. J. Turner, S. zcan, B. Morgan, R. Liang, W. N. Hardy, and D. A. Bonn, Phys. Rev. Lett. **99**, 237003 (2007).
[3] W. Huttema, B. Morgan, P. Turner, W. Hardy, X. Zhou, D. Bonn, R. Liang, and D. Broun, Rev. Sci. Instrum. **77**, 023901 (2006).
[4] X. Zhou et al., Phys. Rev. B **87**, 184512 (2013).
[5] S. Sridhar, J. Appl. Phys. **63**, 159 (1988).
[6] H. M. Altshuler, in *Handbook of Microwave Measurements* (Polytechnic Institute of Brooklyn, Brooklyn, New York, 1963), pp. 495–548.
[7] T. Pereg-Barnea, P. Turner, R. Harris, G. Mullins, J. Bobowski, M. Raudsepp, R. Liang, D. Bonn, and W. Hardy, Phys. Rev. B **69**, 184513 (2004).
[8] C. Truncik, W. Huttema, P. Turner, S. zcan, N. Murphy, P. Carrire, E. Thewalt, K. Morse, A. Koenig, J. Sarrao, et al., Nat. Comm. **4**, 2477 (2013).
[9] R. Liang, P. Dosanjh, D. Bonn, D. Baar, J. Carolan, and W. Hardy, Physica C **195**, 51 (1992).
[10] R. L. S. Kama and, A. Hosseini, D. A. Bonn, and W. N. Hardy, Phys. Rev. B **59**, R8933 (1998).
[11] A. Hosseini, R. Harris, S. Kamal, P. Dosanjh, J. Preston, R. Liang, W. N. Hardy, and D. A. Bonn, Phys. Rev. B **60**, 1349 (1999).
[12] J. Gittleman and B. Rosenblum, J. Appl. Phys. **39**, 2617 (1968).
[13] J. Bardeen and M. J. Stephen, Phys. Rev. **140**, 1197 (1965).
[14] W. F. Vinen and J. J. Niemela, J. Low Temp. Phys. **128**, 167 (2002).
[15] M. Golosovsky, M. Tsindlekht, and D. Davidov, Sup. Sci. Tech. **9**, 1 (1996).
[16] B. Josephson, Phys. Lett. **1**, 251 (1962).
[17] M. Coffey and J. Clem, Phys. Rev. Lett. **67**, 386 (1991).
[18] E. Brandt, Phys. Rev. Lett. **67**, 2219 (1991).
[19] R. Liang, D. Bonn, and W. Hardy, Philosophical Magazine **92**, 2563 (2012).
[20] R. Liang et al., Physica C **383**, 1 (2002).
[21] D. M. Broun, W. A. Huttema, P. J. Turner, S. Ozcan, B. Morgan, R. Liang, W. N. Hardy, and D. A. Bonn, Phys. Rev. Lett. **99**, 237003 (2007).
[22] W. A. Huttema, J. S. Bobowski, P. J. Turner, R. Liang, W. N. Hardy, D. A. Bonn, and D. M. Broun, Phys. Rev. B **80**, 104509 (2009).
[23] D. C. Peets, R.-X. Liang, M. Raudsepp, W. N. Hardy, and D. A. Bonn, J. Cryst. Growth **312**, 344 (2010).
[24] S. Bhattacharya, M. Higgins, and T. Ramakrishnan, Phys. Rev. Lett. **73**, 1699 (1994).
[25] M. N. Kunchur, B. I. Ivlev, D. K. Christen, and J. M. Phillips, Phys. Rev. Lett. **84**, 5204 (2000).
[26] T. Higuchi, S. I. Yoo, and M. Murakami, Phys. Rev. B **59**, 1514 (1999).
[27] R. Harris, P. J. Turner, S. Kamal, A. R. Hosseini, P. Dosanjh, G. K. Mullins, J. S. Bobowski, C. P. Bidinosti, D. M. Broun, R. Liang, et al., Phys. Rev. B **74**, 104508 (2006).
[28] Y. Tsuchiya, K. Iwaya, K. Kinoshita, T. Hanaguri, H. Kitano, A. Maeda, K. Shibata, T. Nishizaki, and N. Kobayashi, Phys. Rev. B **63**, 184517 (2001).
[29] B. Parks et al., Phys. Rev. Lett. **74**, 3265 (1995).
[30] B. Seeber and J. Nickl, Phys. Status Solidi A **15**, 73 (1973).
[31] J. Sonier et al., Phys. Rev. Lett. **79**, 1742 (1997).
